# Supplementary material for: Automatic Data Augmentation via Invariance-Constrained Learning
Source: arXiv:2209.15031 source file (2023-09-15)
Supplement: Supplementary file 1 [file 6_4_appendix_robustness.tex]

\section{Invariance and robustness.}
In this work we motivated invariance from the perspective of generalization, that is, as an underlying property of the data distribution. However, invariance is also sought in order to achieve robustness to covariate shifts that may appear at test-time or deployment~\citep{generalizing-adv-data-aug}, of special relevance in safety and security critical domains \citep{adv-safety}.  Traditionally, the adversarial risk is defined in terms of worst-case additive perturbations bounded on the $L_\infty$ or $L_1$ norm \citep{Szegedy-adv-nn-og, adv-nn-Huang2015, Madry2018TowardsDL}. In  several domains~\citep{adversarial-malware, adversarial-nlp, adversarial-audio} this has been extended to worst-case perturbations under other transformation sets. In computer vision, these include translations~\citep{making-cnn-great-again}, rotations~\citep{madry-spatial-robustness}, color~\citep{adversarial-color} and other semantic transformations~\citep{generalizing-adv-data-aug,semanticadv}. Augmenting the dataset by sampling transformations from an arbitrary distribution does not guarantee that the model will be robust against all transformations, given that the loss is minimized on expectation over the distribution of transformations.  Adversarial training thus aims to minimize the risk under worst-case transformations by generating adversarially perturbed training samples. Since the data distribution may not be invariant to these transformations, a trade-off between robustness and performance also arises~\citep{madry-tradeoff, Dobriban2020ProvableTI}.

Therefore, the invariance-constrained approach can also be used to balance this trade-off and address robustness requirements, that may exist regardless of the natural data distribution. We first describe this setting in Section~\ref{a:rob:Formulation} and then test it on image and pointcloud classification tasks in Sections~\ref{a:rob:description} and \ref{a:rob:results}.

\subsection{Setting}~\label{a:rob:Formulation}
We have worked on the assumption that the underlying distribution of data remains unchanged.
Another possible scenario is to consider there actually exists a mismatch between the training distribution, which we can obtain samples from, and the test distribution. We can further assume that this shift is introduced by the actions of G under some distribution $\mathfrak{G_{test}}$. Since  $\mathfrak{G_{test}}$ is unknown, a common approach is to consider worst-case perturbations
\begin{equation}\label{Adv-loss}
\max_{g \in \mathcal{G}}\ell(h\left(g\mathbf{x}\right), y)).
\end{equation}
In this context, the result of the maximisation over $\matcal{G}$ $\ell_{adv}(h, \mathbf{x}, y)$ is known as the \emph{adversarial loss}. %The adversarial risk has the advantage that, as long as the worst-case perturbations have non-zero mass, it is insensitive to the test distribution.
 %\begin{equation} \tag{SRM-Adv}\label{SRM-Adv}
 %h^*_{adv}\subseteq \operatorname{argmin}_{h \in \mathcal{H}}  R_{adv}(h):=\mathbb{E}_{(\mathbf{x}, y) \sim \mathfrak{D}}[\ell_{adv}(h, \mathbf{x}, y)].
%\end{equation}
Because adversarial robustness may be overly conservative i.e. the worst case perturbation may have a low probability under the test distribution, in practice penalized objectives \citep{goodfellow-adversarial-reg} are used to balance the trade-off between performance and robustness
 \begin{equation}\label{SRM-Adv-gamma}
\operatorname{minimize}_{h \in \mathcal{H}}\;  R(h) + \gamma R_{adv}(h).
\end{equation}

Therefore, the invariance-constrained learning problem that our work addresses can also be formulated with the aim achieving robustness. We now describe particular applications in~\ref{a:rob:description} and include some experiments (Section~\ref{a:rob:results} that show our approach can be advantageous in this setting.

\subsection{Description}~\label{a:rob:description}

\subsection{Results}~\label{a:rob:results}
\subsection{Robustness}

In the case of images we consider a subset of Special Euclidean transformations: the composition of rotations in the range of $\pm 30$ degrees and translations in the range of $\pm 10\%$ of the images' dimension, as in \citep{madry-spatial-robustness}. For pointcloud classification we add a $L_{\infty}$ bounded norm perturbation to the coordinates of each point in the cloud, as in~\cite{pointcloud-adv-extending, pointcloud-adversarial, pointcloud-adversarial-2}. Further details about the setup of distribution shift and adversarial robustness experiments can be found in Appendix~\ref{a:ood-details} and~\ref{a:adversarial-details}, respectively.

\subsubsection{Distribution Shift}

 We consider a \emph{distribution shift} introduced by applying transformations that are sampled from a given probability distribution. We evaluate out-of-distribution accuracy by applying transformations randomly sampled according to a Beta distribution. More details on the experimental setup can be found in Appendix~\ref{a:ood-details}. We compare our approach, which constrains the smoothed adversarial loss, to imposing a constraint on the loss of samples augmented using \emph{the same distribution} of transformations applied on the test set. 

For different levels of the constraint, we find that constraining the \emph{smoothed adversarial} results in a considerably smaller generalization gap using clean test data for the STL dataset. As shown in Figure~\ref{plot:ood:beta-stl10}, it outperforms the beta-constrained model on the original test set. When sampling iid transformations for each image,  the adversarial constrained model also has a better out-of-distribution performance. The performance degradation introduced by the distribution shift is similar for both augmentation distributions, and changes are small compared to the generalization gap on the original test data. %That is, counter-intuitively, constraining the smoothed adversarial loss, which makes no distributional assumptions, can be competitive with using prior knowledge of the distribution of transformations. 

As shown in appendix~\ref{a:results:ood} the CIFAR and Modelnet40~\citep{modelnet40} datasets show a different behaviour. Constraining the adversarial and the augmented loss under the beta distribution used in testing show similar performances both in terms of clean and transformed data. Appendix~\ref{a:results:ood} shows the test accuracy when sampling rotations according to different distributions.
\begin{figure}[h!]
    \centering
     \includegraphics[width=.5\textwidth]{figures/ood/stl10_beta.png}
        \caption{In and Out of distribution accuracy when a distribution shift is introduced applying SE transformations sampled according to a $\beta(0.5, 0.25)$ distribution on test data, using the STL10 dataset. Markers represent the transformation distribution used as a constraint, and the color the value of constraint on the cross entropy loss. In both cases tighter constraints lead to lower clean accuracy, and clean accuracy is highly correlated with OOD accuracy. The smoothed Adversarial results in higher accuracy, both for clean and transformed test data.}
        \label{plot:ood:beta-stl10}
\end{figure}
